# Supplementary material for: Scalable Interpretability via Polynomials
Source: arXiv:2205.14108 source file (2022-10-18)
Supplement: Supplementary file 2 [file ablations.tex]

\section{Ablation Experiments}
\label{sec:appendix_ablation_experiments}
\subsection{Effect of Sharing Bases}
\label{sec:appendix_sharing_bases}
As mentioned i
\subsection{{\sc NeuralSPAM}}
\label{sec:appendix_lrdp_nonlinear}
